# Supplementary material for: Revenue Maximization of Airbnb Marketplace using Search Results
Source: arXiv:1911.05887 source file (2019-11-16)
Supplement: Supplementary file 1 [file appendix.tex]

\begin{comment}




\begin{table}[htbp] %the data here needs to be changed
	\begin{center}
		\caption{Results for setting 1 - Baseline: Home pricing model} 
		\scalebox{1}{
\begin{tabular}{lrrr}
\toprule
{} & Recall &     BR &   w\_BR \\
\midrule
new        &   +7.1\% & -90.6\% & -88.2\% \\
value\_only &   +7.8\% & -81.4\% & -79.1\% \\
%adapt\_CRM  &   0.0\% &   0.0\% &   0.0\% \\
%baseline1  &   7.8\% & 693.2\% & 816.0\% \\
AVG  &   +7.8\% & +693.2\% & -98.7\% \\

\toprule
{} &    pdr & pdr\_high\_p\_low\_b & rev\_potential \\
\midrule
new        & -21.3\% &            +26.4\% &         +55.1\% \\
value\_only & -11.9\% &            +36.5\% &         +63.8\% \\
%adapt\_CRM  &  0.000 &             0.0\% &          0.0\% \\
%baseline1  &  0.574 &            79.6\% &       -561.3\% \\
AVG  & -66.5\% &           -45.2\% &        -32.9\% \\
\bottomrule
\end{tabular}
		}
	\end{center}
\end{table}


\begin{figure}[htb]
\centering
\includegraphics[width=\linewidth]{figures/distributions.png}
\caption{caption.}
\label{fig:qreg}
\end{figure}

\pv{Lets put much more results, we need more insights, you can do new day by day evaluations, you can show few markets, you can show two example of pricing.}

\pv{rev potential 1.5, }


\begin{table}[htbp] %the data here needs to be changed
	\begin{center}
		\caption{Results for New York setting 1} 
		\scalebox{1}{
\begin{tabular}{lrrrrrrrrrrrr}
\toprule
{} & Suggestion Percentage &  BR &  BR\_w &  PDR &   pd\_low\_c &   pd\_high\_c &   pd\_low\_b &   pd\_high\_b &  pd\_hplb &  pd\_lphb &  revenue\_potential\_all &  revenue\_potential\_e \\
\midrule
0 &       0.993 &   0.010 &     0.804 &  0.564 &      0.624 &       0.589 &      0.624 &       0.554 &    0.713 &    0.500 &                 23.022 &               25.426 \\
1 &       1.000 &   0.046 &     1.905 &  0.686 &      0.711 &       0.685 &      0.711 &       0.703 &    0.783 &    0.643 &                 19.164 &               21.250 \\
2 &       0.915 &   0.134 &     4.882 &  0.660 &      0.568 &       0.603 &      0.568 &       0.635 &    0.519 &    0.643 &                 16.935 &               19.819 \\
3 &       1.000 &   1.000 &    45.000 &  1.000 &      1.000 &       1.000 &      1.000 &       1.000 &    1.000 &    1.000 &                -15.715 &              -39.289 \\
4 &       1.000 &   0.000 &     0.000 &  0.136 &      0.078 &       0.192 &      0.078 &       0.189 &    0.078 &    0.143 &                 13.048 &               14.298 \\
\bottomrule




\end{tabular}

		}
	\end{center}
\end{table}







\begin{table}[htbp] %the data here needs to be changed
	\begin{center}
		\caption{Results for San Francisco setting 1} 
		\scalebox{1}{
\begin{tabular}{lrrrrrrrrrrrr}
\toprule
{} &  recall\_new &  BR\_all &  w\_BR\_all &    pdr &   pd\_low\_c &   pd\_high\_c &   pd\_low\_b &   pd\_high\_b &  pd\_hplb &  pd\_lphb &  revenue\_potential\_all &  revenue\_potential\_e \\
\midrule
0 &       0.999 &   0.000 &     0.000 &  0.566 &      0.638 &       0.559 &      0.638 &       0.545 &    0.673 &    0.455 &                 24.309 &               28.941 \\
1 &       1.000 &   0.004 &     0.107 &  0.619 &      0.709 &       0.618 &      0.709 &       0.606 &    0.808 &    0.455 &                 22.242 &               26.077 \\
2 &       0.938 &   0.242 &     8.584 &  0.871 &      0.677 &       0.853 &      0.677 &       0.909 &    0.808 &    0.909 &                 14.499 &               17.523 \\
3 &       1.000 &   1.000 &    35.000 &  1.000 &      1.000 &       1.000 &      1.000 &       1.000 &    1.000 &    1.000 &                -25.075 &              -62.688 \\
4 &       1.000 &   0.000 &     0.000 &  0.149 &      0.071 &       0.088 &      0.071 &       0.121 &    0.038 &    0.182 &                  2.535 &                1.680 \\
\bottomrule
\end{tabular}
		}
	\end{center}
\end{table}



\begin{table}[htbp] %the data here needs to be changed
	\begin{center}
		\caption{Results for 25 Markets: setting 1} 
		\scalebox{1}{
\begin{tabular}{lrrrrrrrrrrrr}
\toprule
{} &  recall\_new &  BR\_all &  w\_BR\_all &    pdr &   pd\_low\_c &   pd\_high\_c &   pd\_low\_b &   pd\_high\_b &  pd\_hplb &  pd\_lphb &  revenue\_potential\_all &  revenue\_potential\_e \\
\midrule
0 &       0.993 &   0.012 &     0.552 &  0.495 &      0.597 &       0.540 &      0.598 &       0.522 &    0.641 &    0.388 &                 17.043 &               18.452 \\
1 &       1.000 &   0.023 &     0.987 &  0.559 &      0.682 &       0.605 &      0.683 &       0.586 &    0.760 &    0.447 &                 17.771 &               19.476 \\
2 &       0.928 &   0.126 &     4.727 &  0.635 &      0.538 &       0.647 &      0.538 &       0.640 &    0.557 &    0.540 &                 10.230 &               11.893 \\
3 &       1.000 &   1.000 &    43.303 &  1.000 &      0.999 &       1.000 &      1.000 &       1.000 &    1.000 &    1.000 &                -21.945 &              -54.863 \\
4 &       1.000 &   0.001 &     0.062 &  0.213 &      0.239 &       0.214 &      0.238 &       0.216 &    0.305 &    0.194 &                  7.806 &                7.975 \\
\bottomrule
\end{tabular}	
}
	\end{center}
\end{table}





\begin{table}[htbp] %the data here needs to be changed
	\begin{center}
		\caption{Results for 25 Markets: setting 2} 
		\scalebox{1}{
\begin{tabular}{lrrrrrrrrrrll}
\toprule
{} &  recall\_new &  BR\_all &  w\_BR\_all &    pdr &   pd\_low\_c &   pd\_high\_c &   pd\_low\_b &   pd\_high\_b &  pd\_hplb &  pd\_lphb &       revenue\_potential\_all &         revenue\_potential\_e \\
\midrule
0 &       0.995 &   0.012 &     0.525 &  0.491 &      0.566 &       0.521 &      0.565 &       0.488 &    0.586 &    0.373 &                      15.176 &                     16.6206 \\
1 &       1.000 &   0.015 &     0.663 &  0.524 &      0.658 &       0.575 &      0.658 &       0.540 &    0.697 &    0.414 &                     16.0257 &                     17.6702 \\
2 &       0.974 &   0.156 &     6.356 &  0.665 &      0.597 &       0.636 &      0.597 &       0.609 &    0.629 &    0.570 &                     10.9951 &                     10.6452 \\
3 &       1.000 &   1.000 &    43.823 &  1.000 &      1.000 &       1.000 &      1.000 &       1.000 &    1.000 &    0.995 &                    -20.3986 &                    -50.9965 \\
4 &       1.000 &   0.001 &     0.046 &  0.238 &      0.171 &       0.208 &      0.170 &       0.211 &    0.211 &    0.230 &  Series([], dtype: float64) &  Series([], dtype: float64) \\
\bottomrule
\end{tabular}
}
	\end{center}
\end{table}






\begin{table}[htbp] %the data here needs to be changed
	\begin{center}
		\caption{Result for one session} 
		\scalebox{1}{
\begin{tabular}{lrrrrrrrrr}
\toprule
{} &  label &  position &  id\_experience &  xgbregressor &  agg\_price\_suggestion &  m\_booking\_price &  price\_sugg &  baseline1 &  rep\_price1 \\
id\_federated\_search                  &        &           &                &               &                       &                  &             &            &             \\
\midrule
013b96f6-6f76-427c-ac2a-ac30202d599e &      0 &        22 &         659908 &     33.809900 &             37.910809 &             45.0 &   21.661458 &          0 &   43.000000 \\
013b96f6-6f76-427c-ac2a-ac30202d599e &      0 &        20 &         600339 &     11.457149 &             12.057514 &             15.0 &   10.510206 &          0 &   15.000000 \\
013b96f6-6f76-427c-ac2a-ac30202d599e &      0 &        30 &         631240 &     62.510110 &             57.421316 &             50.0 &   44.638989 &          0 &   50.000000 \\
013b96f6-6f76-427c-ac2a-ac30202d599e &      0 &        25 &         795659 &     35.231697 &             23.903535 &             85.0 &   85.000000 &          0 &   85.000000 \\
013b96f6-6f76-427c-ac2a-ac30202d599e &      0 &        28 &         395567 &     15.068801 &             18.836001 &             22.0 &   22.000000 &          0 &   22.000000 \\
013b96f6-6f76-427c-ac2a-ac30202d599e &      5 &         3 &         403234 &     40.946150 &             40.130784 &             35.0 &   34.009742 &          0 &   45.700000 \\
013b96f6-6f76-427c-ac2a-ac30202d599e &      1 &        29 &         210126 &     50.343630 &             53.649624 &             50.0 &   55.129804 &          0 &   51.000000 \\
013b96f6-6f76-427c-ac2a-ac30202d599e &      0 &        16 &         659404 &     30.575045 &             42.894909 &             49.0 &   23.254598 &          0 &   49.000000 \\
013b96f6-6f76-427c-ac2a-ac30202d599e &      0 &        18 &         196030 &     34.605892 &             35.649909 &             36.0 &   43.428960 &          0 &   36.666667 \\
013b96f6-6f76-427c-ac2a-ac30202d599e &      0 &        24 &         741158 &     57.290390 &             64.516062 &             60.0 &   97.300487 &          0 &   60.428571 \\
013b96f6-6f76-427c-ac2a-ac30202d599e &      0 &         6 &         180370 &     67.682846 &             63.686329 &             69.0 &   50.778047 &          0 &   69.150000 \\
013b96f6-6f76-427c-ac2a-ac30202d599e &      1 &        35 &         552370 &     13.214139 &             10.254139 &             20.0 &   27.819190 &          0 &   20.000000 \\
013b96f6-6f76-427c-ac2a-ac30202d599e &      0 &         7 &         396428 &     15.002605 &             13.142042 &             20.0 &    7.078610 &          0 &   16.100000 \\
013b96f6-6f76-427c-ac2a-ac30202d599e &      0 &        11 &          95224 &     29.489925 &             31.442823 &             30.0 &   21.442116 &          0 &   30.055556 \\
013b96f6-6f76-427c-ac2a-ac30202d599e &      0 &        19 &         762752 &     29.355541 &             33.864496 &             45.0 &   45.000000 &          0 &   47.750000 \\
013b96f6-6f76-427c-ac2a-ac30202d599e &      0 &        13 &         122450 &     34.245617 &             34.156529 &             35.0 &   31.025688 &          0 &   35.142857 \\
013b96f6-6f76-427c-ac2a-ac30202d599e &      0 &         2 &         806898 &     21.667425 &             21.022064 &             22.0 &   22.000000 &          0 &   22.000000 \\
013b96f6-6f76-427c-ac2a-ac30202d599e &      0 &        26 &         110065 &     57.535820 &             58.759954 &             50.0 &   41.099993 &          0 &   54.069767 \\
013b96f6-6f76-427c-ac2a-ac30202d599e &      1 &        43 &         841079 &     57.406063 &             49.293272 &             50.0 &   50.000000 &          0 &   75.000000 \\
013b96f6-6f76-427c-ac2a-ac30202d599e &      1 &        10 &         167554 &     91.033110 &             90.196121 &             89.0 &   69.498931 &          0 &   78.222222 \\
013b96f6-6f76-427c-ac2a-ac30202d599e &      0 &        17 &          73865 &     75.653540 &             76.003472 &             75.0 &   63.980311 &          0 &   75.888889 \\
013b96f6-6f76-427c-ac2a-ac30202d599e &      0 &        14 &          98988 &     34.353096 &             33.949383 &             35.0 &   25.831834 &          0 &   36.545455 \\
013b96f6-6f76-427c-ac2a-ac30202d599e &      0 &         8 &         157851 &     32.055720 &             32.540911 &             35.0 &   29.412225 &          0 &   35.478261 \\
013b96f6-6f76-427c-ac2a-ac30202d599e &      0 &         4 &         445486 &     47.727390 &             50.398310 &             49.0 &   37.384096 &          0 &   36.769231 \\
013b96f6-6f76-427c-ac2a-ac30202d599e &      0 &        27 &         762749 &     31.118086 &             34.054799 &             45.0 &   45.602107 &          0 &   46.000000 \\
013b96f6-6f76-427c-ac2a-ac30202d599e &      0 &         5 &         754915 &     15.821740 &             13.674172 &             14.0 &   14.773190 &          0 &   14.000000 \\
013b96f6-6f76-427c-ac2a-ac30202d599e &      0 &        23 &         563063 &    129.201400 &            122.982768 &            129.0 &  121.652012 &          0 &  130.750000 \\
013b96f6-6f76-427c-ac2a-ac30202d599e &      0 &         0 &         139532 &     43.394257 &             47.125908 &             45.0 &   32.081841 &          0 &   45.833333 \\
013b96f6-6f76-427c-ac2a-ac30202d599e &      2 &        12 &         692852 &     47.236084 &             39.921873 &             40.0 &   32.067482 &          0 &   47.625000 \\
013b96f6-6f76-427c-ac2a-ac30202d599e &      0 &        15 &         185095 &     41.747920 &             52.241706 &             49.0 &   54.436554 &          0 &   50.000000 \\
013b96f6-6f76-427c-ac2a-ac30202d599e &      0 &         1 &         298126 &     83.457130 &             81.312756 &             80.0 &  164.451041 &          0 &   80.985294 \\
013b96f6-6f76-427c-ac2a-ac30202d599e &      0 &        21 &         500361 &     29.234898 &             30.386841 &             30.0 &   26.808546 &          0 &   29.781250 \\
013b96f6-6f76-427c-ac2a-ac30202d599e &      0 &         9 &         577058 &     25.273535 &             29.684188 &             51.0 &   33.914882 &          0 &   45.439103 \\
\bottomrule
\end{tabular}

}
	\end{center}
\end{table}






\end{comment}
